# Supplementary material for: Deep is a Luxury We Don't Have
Source: arXiv:2208.06066 source file (2022-08-11)
Supplement: Supplementary file 1 [file appendix_introduction.tex]

\section{Appendix: Introduction}\label{sec:app_introduction}
Transformers are already ubiquitous for medical images processing. Yet, recent literature avoid tackling the computational cost by using low resolution inputs. Conversely, our architecture, HCT, is designed for high resolution input,~\ie  2-3K pixels per dimension. This is a key difference between our approach and recent literature. In addition, we evaluate the effective receptive field of HCT. This evaluation is essential to verify the claim that transformers are better in modeling long-range dependencies. The following paragraphs review the transformer literature in medical imaging. These approaches are grouped by their applications.\\

\topic{Medical Image Classification~\cite{matsoukas2021time}}

\topic{Medical Image Segmentation~\cite{valanarasu2021medical,gao2021utnet,xie2021cotr,wang2021transbts,zhang2021transfuse}} These approaches uses transformer in U/V-Net~\cite{ronneberger2015u,milletari2016v} architecture to segment medical images. For instance, Xie~\etal~\cite{xie2021cotr} have leveraged transformers for 3D Medical Image Segmentation. The proposed architecture, CoTr, consumes low resolution inputs (\eg 48×192×192), while UTNet~\cite{gao2021utnet} consumes 256x256. CoTr uses Multi-layer perceptron (MLP) and explicit positional encoding. This reduces the architecture agility for different input resolutions. Conversely, HCT uses conv layers on top of attention layers. This strategy eliminates the need for explicit positional encoding as reported by recent literature~\cite{wu2021cvt}. Finally, Xie~\etal~\cite{xie2021cotr} evaluation leverages one dataset with 30 labeled CT scans, while our evaluation leverages two larger datasets. Indeed, segmentation annotations are more expensive than classification annotations. Still, our comparably large datasets raises confidence in our findings.

\topic{Image Denoising~\cite{zhang2021transct,luthra2021eformer,wang2021ted}} Zhang~\etal~\cite{zhang2021transct} have proposed transformers to enhance the quality of low dose computed tomography (LDCT) images. The proposed architecture, TransCT, crosses attention between low frequency and high frequency bands of the image. TransCT takes low resolution inputs,~\ie 512x512. Furthermore, Our proposed AC block is simple compared to the encoder-decoder in TransCT.
Finally, a single dataset~\cite{mccollough2017low} of total 30 labeled LDCT images (10 training and 20 testing) is used for evaluating TransCT.
