# Supplementary material for: Deep is a Luxury We Don't Have
Source: arXiv:2208.06066 source file (2022-08-11)
Supplement: Supplementary file 2 [file appendix_ablation_study.tex]

\section{Appendix: Ablation Study}\label{sec:app_ablation_study}
Receptive field before and after training
