# Supplementary material for: Deep is a Luxury We Don't Have
Source: arXiv:2208.06066 source file (2022-08-11)
Supplement: Supplementary file 3 [file appendix_experiments.tex]

\section{Appendix}\label{sec:app_experiments}

%\topic{Further dataset details}In OPTIMAM, an image is labeled as malignant (positive) if it has a malignant biopsy in the corresponding breast within 12 months of the screening exam. Images labeled as non-malignant (negative) are required to have either a benign biopsy within 12 months of the screening exam or 24 months of non-malignant imaging follow-up. Images that violate the above criteria are excluded from both training and inference.

\topic{Further Technical Details} 
For training the patch mode, we sampled positive patches from malignant images with a bounding box annotation of the malignant tissue.  Each positive patches is centered inside the bounding box. We sampled negative patches from non-malignant images. Each negative patch is randomly centered within the breast tissue. All patches are $512\times512$.

\newcommand{\ahscale}{0.24} 
\newcommand{\awscale}{0.20} %wscale = \hscale * 2560 / 3328 
\begin{table}[t]
	\scriptsize
	\centering
	\caption{Effective receptive field (ERF) analysis for GMIC (Blue), Def-GMIC (Red), and HCT (Orange). This ERF is generated using $N=100$ randomly sample left and right breasts ($1^{\text{st}}$ column), right breasts ($2^{\text{nd}}$ column), and left breasts ($3^{\text{rd}}$ column). We only report the aggregated ERF across rows only for brevity.}
	\label{tab:receptive_field_analysis_def_gmic}
	\setlength{\tabcolsep}{2pt}
	\begin{tabular}{@{}ccc@{}}
		\toprule
		Left and Right & Right& Left\\
		\midrule
		\includegraphics[width=\awscale\linewidth,height=\ahscale\linewidth]{./figures\Ver/both_gmic_dgmic_i_pmag_cols.png} &
		\includegraphics[width=\awscale\linewidth,height=\ahscale\linewidth]{./figures\Ver/right_gmic_dgmic_i_pmag_cols.png} &
		\includegraphics[width=\awscale\linewidth,height=\ahscale\linewidth]{./figures\Ver/left_v2_gmic_dgmic_i_pmag_cols.png}\\
		\bottomrule
	\end{tabular}
\end{table}

Algorithm~\ref{alg:ac_block} presents the forward pass of the proposed AC block. This implementation follows GMIC's implementation\footnote{\href{https://github.com/nyukat/GMIC/blob/e8f539f2515f648cdd3a7c624363abdd3f4f973a/src/modeling/modules.py\#L51}{src/modeling/modules.py\#L51}}. GMIC adapts  the ``pre-activation'' style~\cite{he2016identity} in contrast to conventional wisdom of ``post-activation''. Yet, ``pre-activation'' has been promoted in literature~\cite{he2016identity,touvron2021going} to improve generalization.

\begin{algorithm}[t]
		\tiny
	\caption{The proposed AC block's forward pass.}\label{alg:ac_block}
		\tiny
		%\centering
		\begin{tabular}{@{}cc@{}}
			\begin{lstlisting}[language=Python]
def forward(self, x):
		residual = x

		out = self.bn1(x)
		out = self.relu(out)
		if self.downsample is not None:
			residual = self.downsample(out)		
		out = self.linear_attention(out)
		
		out += x
		
		out = self.bn2(out)
		out = self.relu(out)
		# This conv controls both
		# resolution and # of channels
		out = self.conv2(out)

		out += residual
		return out\end{lstlisting}
		&
		\begin{lstlisting}[language=Python]
def linear_attention(self, x):
		bz, num_chns, rows, cols = x.shape
		
		## Reshape for Transformer
		x = x.view(bz, num_chns, -1) 
		x = x.permute(0, 2, 1)
		
		# We recommend Performer-RELU. Yet,
		# other linear approximations work
		q = self.attention(x)
		
		## Reshape for CNNs
		q = q.permute(0, 2, 1)
		q = q.view(bz, -1, rows, cols)  
		return q
		
		
		
		\end{lstlisting}
		\end{tabular}
\end{algorithm}
